# Supplementary material for: Persistent Homology for Effective Non-Prehensile Manipulation
Source: arXiv:2202.02937 source file (2022-02-07)
Supplement: Supplementary file 1 [file 10_appendix.tex]

\section{Appendix}
\label{sec:appendix}
